# Supplementary material for: Monitoring Hyperproperties
Source: arXiv:1807.00758 source file (2018-07-02)
Supplement: Supplementary file 1 [file appendix.tex]

\section{Tables}
We extended Table~\ref{formulaanalysis} with $\hyperltl$ formulas used in a case study in~\cite{conf/cav/FinkbeinerRS15} to verify versions of the bakery protocol (symm1 - symm2) and error resisting codes (Ham).
\begin{table}[]
	\centering
	\caption{Formula Analysis for universally quantified hyperproperties studied in the literature. Each property has been checked in under $1 s$.}
	\label{formulaanalysis-extended}
	\begin{tabular}{ll|l|l|l|}
		\cline{3-5}
		&                                                                                                                                                                                                                                                                                                                                                                                                                                                                    & symm & trans & refl \\ \hline
		\multicolumn{1}{|l|}{ObsDet1}     & $\forall \pi. \forall \pi'.\; \G (I_{\pi} = I_{\pi'}) \rightarrow \G (O_{\pi} = O_{\pi'})$                                                                                                                                                                                                                                                                                                                                                             &  \cmark    &    \xmark   &  \cmark    \\ \hline
		\multicolumn{1}{|l|}{ObsDet2}     & $\forall \pi. \forall \pi'.\; (I_{\pi} = I_{\pi'}) \rightarrow \G (O_{\pi} = O_{\pi'})$                                                                                                                                                                                                                                                                                                                                                                &  \cmark    &    \xmark   &  \cmark      \\ \hline
		\multicolumn{1}{|l|}{ObsDet3}     & $\forall \pi. \forall \pi'. O_\pi = O_\pi' \W I_\pi \neq I_\pi'$                                                                                                                                                                                                                                                                                                                                                                                                   &  \cmark    &    \xmark   &  \cmark      \\ \hline
		\multicolumn{1}{|l|}{QuantNoninf} & $\forall \pi_0 \ldots \forall \pi_{c}.~\neg ((\bigwedge_i I_{\pi_i} = I_{\pi_0}) \wedge \bigwedge_{i \neq j} O_{\pi_i} \neq O_{\pi_j})$                                                                                                                                                                                                                                                                                                                            &  \cmark    &    \xmark   &  \cmark      \\ \hline
		\multicolumn{1}{|l|}{Ham}         & \begin{tabular}[c]{@{}l@{}}$\forall \pi.\; \forall \pi'.\; F (\bigvee_{i\in I} \neg (i_\pi \leftrightarrow i_{\pi'})) \rightarrow \neg \mathit{Ham}_O(d-1,\pi,\pi')$\\ $\mathit{Ham_O}\coloneqq \mathit{Ham_O}(-1,\pi,\pi') = \mathit{false}$ and\\ $\mathit{Ham_O}(d,\pi,\pi') = (\bigwedge_{o\in O} o_\pi \leftrightarrow o_{\pi'})$ \\       $\W (\bigvee_{o\in O} \neg (o_\pi \leftrightarrow o_{\pi'}) \wedge \X\;\mathit{Ham_O}(d-1,\pi,\pi'))$\end{tabular} &  \cmark    &    \xmark   &  \cmark      \\ \hline
		\multicolumn{1}{|l|}{Symm1}       & \begin{tabular}[c]{@{}l@{}}$\forall \pi. \forall \pi'. \G (\mathit{sym}(\mathit{sel}_\pi, \mathit{sel}_{\pi'}) \wedge pause_\pi = pause_{\pi'})$\\ $\rightarrow \G(\mathit{pc}(0)_\pi = \mathit{pc}(1)_{\pi'} \wedge \mathit{pc}_\pi = \mathit{pc}(0)_{\pi'})$\end{tabular}                                                                                                                                                                                        &  \xmark    &    \xmark   &  \cmark      \\ \hline
		\multicolumn{1}{|l|}{Symm2}       & \begin{tabular}[c]{@{}l@{}}$\forall \pi. \forall \pi'. \G (\mathit{sym}(\mathit{sel}_\pi, \mathit{sel}_{\pi'}) \wedge pause_\pi = pause_{\pi'}$\\ $\wedge \mathit{sel}_\pi < 3 \wedge \mathit{sel}_{\pi'} < 3)$\\ $\rightarrow \G(\mathit{pc}(0)_\pi = \mathit{pc}(1)_{\pi'} \wedge \mathit{pc}_\pi = \mathit{pc}(0)_{\pi'})$\end{tabular}                                                                                                                         &  \xmark    &    \xmark   &  \xmark      \\ \hline
		\multicolumn{1}{|l|}{Symm3}       & \begin{tabular}[c]{@{}l@{}}$\forall \pi. \forall \pi'. \G (\mathit{sym}(\mathit{sel}_\pi, \mathit{sel}_{\pi'}) \wedge pause_\pi = pause_{\pi'})$\\ $\wedge \mathit{sel}_\pi < 3 \wedge \mathit{sel}_{\pi'} < 3 \wedge \mathit{sym}(\mathit{symbreak}_\pi,\mathit{symbreak}_{\pi'})$\\ $\rightarrow \G(\mathit{pc}(0)_\pi = \mathit{pc}(1)_{\pi'} \wedge \mathit{pc}_\pi = \mathit{pc}(0)_{\pi'})$\end{tabular}                                                     &  \xmark    &    \xmark   &  \xmark    \\ \hline
		
		\multicolumn{1}{|l|}{ConfMan} &\begin{tabular}[c]{@{}l@{}}$\forall \pi \forall \pi' \ldot \big((\neg pc_\pi \wedge pc_{\pi'}) \rightarrow \X\G (s_\pi \rightarrow \X v_{\pi'})\big)$\\ $\wedge \big((pc_{\pi} \wedge pc_{\pi'}) \rightarrow \X\G (v_\pi \leftrightarrow v_\pi')\big)$\end{tabular} &  \xmark    &    \xmark   &  \xmark \\ \hline
		
		\multicolumn{1}{|l|}{EQ} &\begin{tabular}[c]{@{}l@{}}$\forall \pi. \forall \pi' \ldot \G (a_\pi \leftrightarrow a_{\pi'})$\end{tabular} &  \cmark    &    \cmark   &  \cmark \\ \hline
	\end{tabular}
\end{table}
